# Supplementary material for: Metal-Insulator Transition and Pseudogap in Bi$_{1.76}$Pb$_{0.35}$Sr$_{1.89}$CuO$_{6+\delta}$ High-$T_c$ Cuprates
Source: arXiv:1608.06352 source file (2016-09-03)
Supplement: Supplementary file 1 [file bi2201-supp.pdf]

# Supplementary Material

## 1) Bulk electronic properties of Bi(Pb)2201 samples studied by $\mu$SR

Single crystalline samples of $Bi_{1.76}Pb_{0.35}Sr_{1.89}CuO_{6+\delta}$ were prepared by floating-zone method [1], where Bi was partially substituted with Pb to suppress the modulation on BiO planes [2]. The Pb substitution also provided the great advantage for $\mu$SR that the upper critical field ($B_{c2}$) was much reduced from that in $Ba_2Sr_{2-x}La_xCuO_{6+\delta}$ ($\sim$30 T) with a trade-off of $T_c$ (nearly halfway down from the latter). The carrier doping was attained by controlling oxygen content (annealing under appropriate conditions) instead of La substitution for Sr to minimize a perturbation to $CuO_2$ plane from random strain. The hole carrier concentration was estimated from the $T_{\rm c}$ vs $p$ mapping for the superconducting samples [3], whereas those situated at both ends of the $T_{\rm c}$ dome (HLD and NSOD, $T_{\rm c} = 0$), was evaluated by the Hall coefficient measurements [4,5].

Table 1: Superconductive transition temperatures ($T_{\rm c}$), hole concentration ($p$), and irreversibility field ($B_{irr}$, at 2 K) of the (Bi,Pb)2201 samples studied by $\mu$SR, where $p$ was estimated from the $T_{\rm c}$ vs $p$ mapping [3] (for HLD and NSOD, it was directly estimated by the Hall coefficient measurement [4,5]), and $B_{\rm irr}$ was deduced from magnetization measurement.

| Label | | $T_c$ | $p$ | $B_{\rm irr}$(2 K) |
|---|---|---|---|---|
| HLD | (Heavily lightly doped) | 0 | 0.09(1) | - |
| LD | (Lightly doped) | $<$ 2 K | 0.10 | - |
| HUD | (Heavily underdoped) | 4.7 K | 0.12 | - |
| SUD | (Slightly underdoped) | 17.2 K | 0.14 | - |
| OPT | (Optimally doped) | 19.4 K | 0.16 | 5.5 T |
| OD | (Overdoped) | 15.3 K | 0.185 | 3.5 T |
| HOD | (Heavily overdoped) | 4.8 K | 0.195 | 0.45 T |
| NSOD | (Non-SC overdoped) | 0 | 0.205(5) | - |

## 2) Muon sites and hyperfine parameters

The muon sites were estimated by numerical simulation using the VASP code (Vienna Ab-initio Simlation Package). The Hartree potential was calculated for the given atomic configuration of Bi2201 to locate the candidate sites by the potential minima for the unit positive charge mimiking the interstitial muon, and the hyperfine parameters for the paramagnetic state were evaluated for the respective site by calculating the second moments of the magnetic dipole tensor,

$$A_\mu = \left[\frac{2}{3}\sum_j \langle|\hat{\mathbf{A}}_j\boldsymbol{\mu}_j|\rangle^2\right]^{1/2}, \quad (1)$$

for the possible muon sites; $\hat{\mathbf{A}}_j$ is expressed as

$$\hat{\mathbf{A}}_j = \frac{1}{r_j^3}\left(\frac{3\alpha_j\beta_j}{r_j^2} - \delta_{\alpha\beta}\right) \quad (\alpha, \beta = x, y, z). \tag{2}$$

The summation is done to determine the contribution of the $j$-th Cu moments $\boldsymbol{\mu}_j$ located at $\boldsymbol{r}_j = (x_j, y_j, z_j)$ from a given muon site. The result is summarized in the following Table 2, where the ratio of hyperfine parameters between those associated with Site-A and B (showing the lowest potential energy) is in good correspondence with the ratio of the muon Knight shift observed experimentally. This led to the assignment of $A_{\mu(1)}$ to Site-B and $A_{\mu(2)}$ to Site-A, respectively.

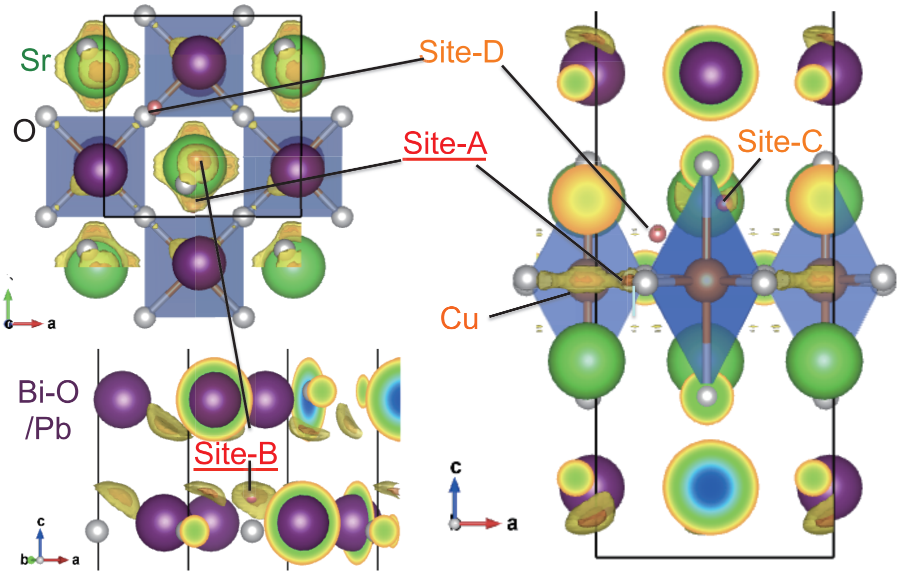


Suppl. Fig. 1: Possible muon sites in Bi2201 cuprates identified as the minima of the Hartree potential calculated by the VASP code. (Illustration drawn by VESTA [6].) For the relevant parameters for the respective site, see Table 2.

Table 2: Lattice coordinates and hyperfine parameters for the possible muon sites. Site-A and -B were assigned to those corresponding to two singals observed in the $\mu$SR experiment.

| Site | Coordinate | O$\mu$ bond length (nm) | Energy (eV) | $A_\mu$ (T/$\mu_B$) | |
|---|---|---|---|---|---|
| A | (0.457 0.055 0.250) | 0.1350 | −9.28 | −0.3373 | $A_{\mu(2)}$ |
| B | (0.470 0.285 0.465) | 0.1146 | −9.24 | +0.0646 | $A_{\mu(1)}$ |
| C | (0.540 0.845 0.320) | 0.1140 | −9.06 | +0.2113 | – |
| D | (0.258 0.545 0.292) | 0.1146 | −8.87 | +0.0876 | – |

### 3) Scaling relation between $K_1(T)$ and $K_2(T)$

Because of the small magnitude of the observed muon Knight shift for two precession

signals [$K_1(T)$ and $K_2(T)$] respectively attributed to different muon sites, we examined the scaling of these two quantities to assess the confidence level of the conclusions drawn from them. As is found in Suppl. Fig. 2(a), $K_1(T)$ vs $K_2(T)$ plot exhibits deviation from the expected linear relation at both high and low temperature ends (upper and lower sides, respectively in terms of $K_2$ axis) due to the reasons discussed in the main text, while each data set falls on a line over an intermediate region from which the ratio $K_2/K_1$ is deduced (see Table 3). Various offset terms common to these two shifts can be eliminated by subtracting one from another (e.g., $K_1 - K_2$), so that the difference would serve as a better variable to examine the mutual linearity of $K_i$. Suppl. Figs. 2(b) and 2(c) shows that even $K_1$ (much smaller than $K_2$) exhibits good linearity with $K_1 - K_2$, where the deviation for the region $K_1 - K_2 \leq$ 50–100 ppm is attributed to the Lorentz demagnetization which is induced by the uniform susceptibility of the samples showing a Curie-Weiss like divergent behavior (due to impurities) at low temperatures.

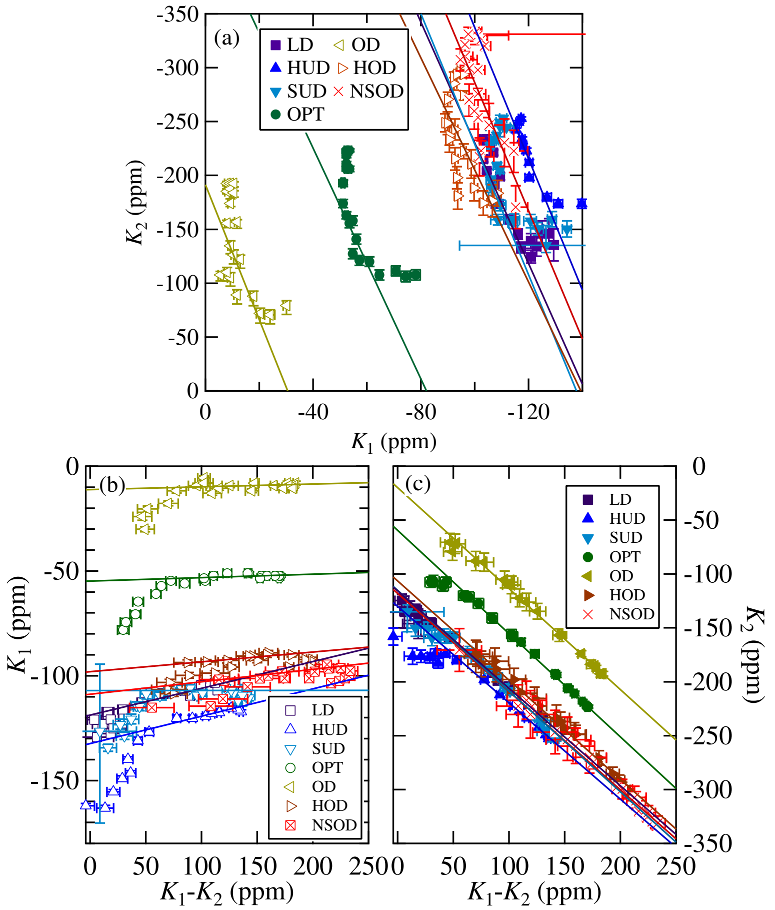


Suppl. Fig. 2: Muon Knight shift $K_i(T)$ ($i = 1, 2$) plotted in three different fashions, (a) $K_1$ vs $K_2$, (b) $K_1$ vs $K_1 - K_2$, and (c) $K_2$ vs $K_1 - K_2$. (No data exists for HLD sample.)

Table 3: Ratio $K_2/K_1$ for the respective samples deduced from curve fits over the intermediate range where a linear relation is observed [shown by solid lines in Suppl. Fig. 2(a)].

| Label | | $K_2/K_1$ |
|---|---|---|
| LD | (Lightly doped) | $-5.6 \pm 0.3$ |
| HUD | (Heavily underdoped) | $-6.1 \pm 0.4$ |
| SUD | (Slightly underdoped) | $-6.0 \pm 0.9$ |
| OPT | (Optimally doped) | $-5.4 \pm 1.1$ |
| OD | (Overdoped) | $-6.2 \pm 0.3$ |
| HOD | (Heavily overdoped) | $-5.2 \pm 1.1$ |
| NSOD | (Non-SC overdoped) | $-5.9 \pm 1.0$ |

## References


1. I. Chong, T. Terashima, Y. Bando, M. Takano, Y. Matsuda, T. Nagaoka and K. Kumagai, Physica C **290**, 57 (1997).

2. Y. Ikeda, Z. Hiroi, H. Ito, S. Shinomura, M. Takano and Y. Bando, Physica C **165** 189 (1990).

3. K. Kudo, N. Okumura, Y. Miyoshi, T. Nishizaki, T. Sasaki and N. Kobayashi, J. Phys. Soc. Jpn. **78**, 084722 (2009).

4. S. Ono, S. Komiya, and Y. Ando, Phys. Rev. B **75** 024515 (2007).

5. Y. Ando, Y. Hanaki, S. Ono, T. Murayama, K. Segawa, N. Miyamoto, and S. Komiya, Phys. Rev. B **61**, R14956 (2000); *ibid.* **63**, 069902(E) (2001).

6. K. Momma and F. Izumi, J. Appl. Crystallogr. **44**, 1272 (2011).
